# Supplementary material for: Simulation and Learning for Urban Mobility: City-scale Traffic Reconstruction and Autonomous Driving
Source: arXiv:1908.06131 source file (2019-08-05)
Supplement: Supplementary file 1 [file appendix.tex]

\begin{figure*}[hb]
\centering
\includegraphics[width=\textwidth]{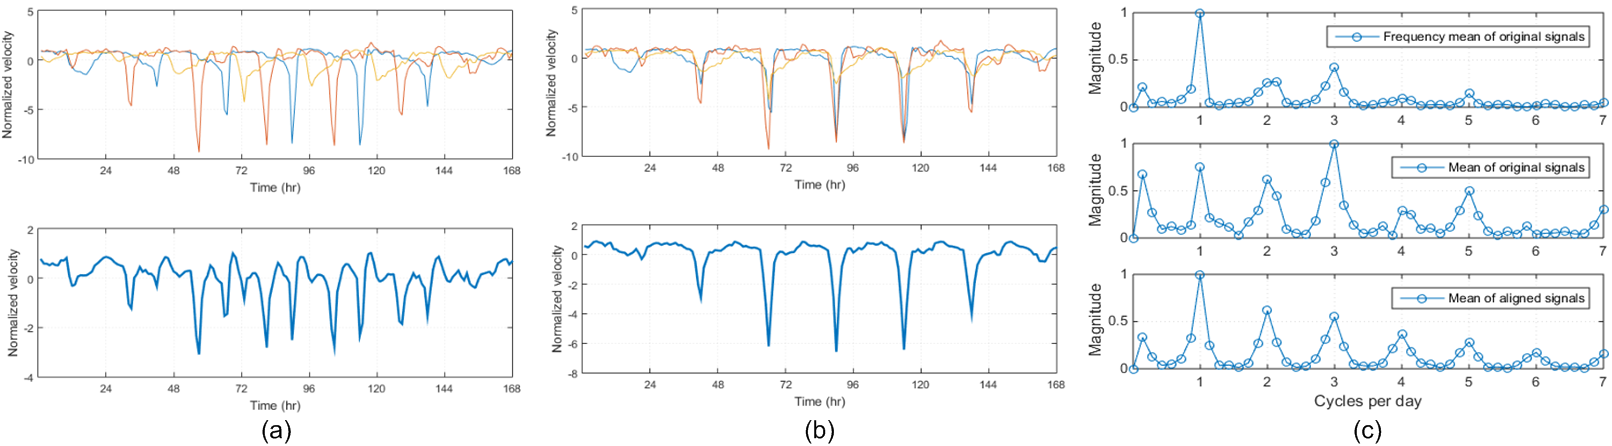}
\caption{(a) Several loop-detector signals are plotted showing phase shifts among them (top panel); the average signal of phase varied loop-detector signals (bottom panel). (b) Aligned loop-detector signals according to their phase responses (top panel); the average signal of aligned loop-detector signals (bottom panel). (c) Averaged frequency of phase varied loop-detector signals showing several frequencies are getting degraded (top panel); frequency of the averaged but phase varied loop-detector signals showing incorrect magnitude ratios (center panel); frequency of the averaged aligned signals with prominent frequencies and corresponding magnitude ratios (bottom panel).}
\label{fig:filter}
\end{figure*}

\subsection{Filter Design}
\label{section:appendix_filter_design}

Traffic exhibits periodic patterns. This phenomenon can be seen from the example loop-detector data in Figure 6 in the main text. Referring to the weekly data from a loop detector as a loop-detector signal, we have observed that such a signal can be approximated by a small set of Fourier coefficients while the energy and periodic structure are largely retained. This observation inspired us to develop a frequency domain filter that consists of most dominant frequency components. 

One way of constructing such a filter is to transform all loop-detector signals to the frequency domain and take the average of all frequency components. While this approach can expect to reduce the embedded white noise, it doesn't consider other types of noise in the data. This is illustrated in the top panel of Figure~\ref{fig:filter}\textbf{(c)}: the most significant frequency component is captured while other harmonics are reduced to various degrees. 

Considering time-domain only methods, a na\"{i}ve approach is to get the average signal, transform it to the frequency domain, and analyze its frequency components. Though this is a straightforward way in dealing with univariate and multivariate data, the resulting signal could be a poor summary of original signals both in the time domain (Figure~\ref{fig:filter}\textbf{(a)}) and in the frequency domain (Figure~\ref{fig:filter}\textbf{(c)} middle panel). The reason is that this approach does not take the phase variability into account. Due to these reasons, we align signals in the time domain, calculate the average signal, transform it to the frequency domain, and extract its major frequencies (see Figure~\ref{fig:filter}\textbf{(b)} and Figure~\ref{fig:filter}\textbf{(c)} bottom panel). As a result, we obtain both important frequency components and their corresponding magnitudes in the right ratio. The frequency-domain version of this signal then serves as our filter.

%To evaluate the effectiveness of our filter, we divide loop-detector signals into a training set and a testing set. We construct the filter using the training set and apply it on each signal in the testing set (Figure \ref{filter-loop}). As results, our filter can indeed extract important frequencies and resemble original signals very well.
